# Supplementary material for: Men Also Like Shopping: Reducing Gender Bias Amplification using Corpus-level Constraints
Source: arXiv:1707.09457 source file (2017-07-29)
Supplement: Supplementary file 1 [file appendix.tex]

\begin{table}
\centering
    \begin{tabular}{C{2cm} C{2cm} C{2cm} C{2cm}}
    % \hline
        \bf       &  \bf Mv  & \bf Dt &  \bf Acc \\ \hline
        n-\alg-dev  &  65  &  22.09 &  0.2407\\
        \alg-dev     &  44  & 19.094 &   0.2401\\
        n-\alg-test &  70 &    22.31 &  0.2414\\
        \alg-test    &  55 &   21.15 &  0.2411\\
    \end{tabular}
    \caption{\jy{Statistic results for margin 0.13}}
    \label{tab:gender_ratio_number_0.13}
\end{table}

\begin{figure*}[!h]
    \centering
    \hspace{-30pt}
       \begin{subfigure}[b]{0.25\textwidth}
        \includegraphics[width=\linewidth]{figures/imSitu_gender_ratio_beforeLR.pdf}
        \caption{Gender ratio on training and dev without LR.}
        \label{fig:gender_ratio_beforeLR0}
    \end{subfigure}
    %   \hspace{-16pt}
    \begin{subfigure}[b]{0.25\textwidth}
        \includegraphics[width=\linewidth]{figures/imSitu_gender_ratio_afterLR.pdf}
        \caption{Gender ratio on training and dev with LR. }
        \label{fig:gender_ratio_afterLR0}
    \end{subfigure}
    \begin{subfigure}[b]{0.25\textwidth}
        \includegraphics[width=\linewidth]{figures/imSitu_gender_ratio_test_beforeLR.pdf}
        \caption{Gender ratio  on training and test without LR.}
        \label{fig:test_gender_ratio_beforeLR0}
    \end{subfigure}
    %   \hspace{-16pt}
    \begin{subfigure}[b]{0.25\textwidth}
        \includegraphics[width=\linewidth]{figures/imSitu_gender_ratio_test_afterLR.pdf}
        \caption{Gender ratio on training and test with LR. }
        \label{fig:test_gender_ratio_afterLR0}
    \end{subfigure}
    \caption{Gender biases in the visual SRL system. We set the constraints that the gender ratio we predicted should be within some margin to the training ratio. We can see that after Lagrangian Relaxation, most of the verbs become satisfied to these constraints.} 
    \label{fig:imSitu_gender_ratio0}
\end{figure*}

\begin{figure*}[!h]
    \centering
    \hspace{-30pt}
       \begin{subfigure}[b]{0.26\textwidth}
        \includegraphics[width=\linewidth]{figures/imSitu_man_verb_ratio_beforeLR.pdf}
        \caption{Man: verb ratio in dev dataset without LR.}
        \label{fig:man_dev_verb_ratio_beforeLR0}
    \end{subfigure}
    %   \hspace{-16pt}
    \begin{subfigure}[b]{0.26\textwidth}
        \includegraphics[width=\linewidth]{figures/imSitu_man_verb_ratio_afterLR.pdf}
        \caption{Man: verb ratio in dev data with LR. }
        \label{fig:man_dev_verb_ratio_afterLR0}
    \end{subfigure}
    %   \hspace{-16pt}
    \begin{subfigure}[b]{0.26\textwidth}
        \includegraphics[width=\linewidth]{figures/imSitu_man_test_verb_ratio_beforeLR.pdf}
        \caption{Man: verb ratio in test dataset without LR. }
        \label{fig:man_test_verb_ratio_beforeLR0}
    \end{subfigure}
    %   \hspace{-16pt}
    \begin{subfigure}[b]{0.26\textwidth}
        \includegraphics[width=\linewidth]{figures/imSitu_man_test_verb_ratio_afterLR.pdf}
        \caption{Man: verb ratio in test dataset with LR. }
        \label{fig:man_test_verb_ratio_afterLR0}
    \end{subfigure}
    
    \hspace{-40pt}
       \begin{subfigure}[b]{0.26\textwidth}
        \includegraphics[width=\linewidth]{figures/imSitu_woman_verb_ratio_beforeLR.pdf}
        \caption{Woman: verb ratio in dev dataset without LR.}
        \label{fig:woman_dev_verb_ratio_beforeLR0}
    \end{subfigure}
    %   \hspace{-16pt}
    \begin{subfigure}[b]{0.26\textwidth}
        \includegraphics[width=\linewidth]{figures/imSitu_woman_verb_ratio_afterLR.pdf}
        \caption{Woman: verb ratio in dev data with LR. }
        \label{fig:woman_dev_verb_ratio_afterLR0}
    \end{subfigure}
    %   \hspace{-16pt}
    \begin{subfigure}[b]{0.26\textwidth}
        \includegraphics[width=\linewidth]{figures/imSitu_woman_test_verb_ratio_beforeLR.pdf}
        \caption{Woman: verb ratio in test dataset without LR. }
        \label{fig:woman_test_verb_ratio_beforeLR0}
    \end{subfigure}
    %   \hspace{-16pt}
    \begin{subfigure}[b]{0.26\textwidth}
        \includegraphics[width=\linewidth]{figures/imSitu_woman_test_verb_ratio_afterLR.pdf}
        \caption{Woman: verb ratio in test dataset with LR. }
        \label{fig:woman_test_verb_ratio_afterLR0}
    \end{subfigure}
    \caption{Verb ratio predicted in the visual SRL system. We set the constraints that the verb ratio   should be within some margin to the training ratio. We can see that after Lagrangian Relaxation, many of the verbs become satisfied to these constraints.} 
    \label{fig:imSitu_man_verb_ratio}
\end{figure*}

\begin{figure*}[!h]
    \centering
    \hspace{-30pt}
       \begin{subfigure}[b]{0.25\textwidth}
        \includegraphics[width=\linewidth]{figures/imSitu_mean_gender_ratio_dev_50_013_01.pdf}
        \caption{Mean gender ratio on training and dev without LR.}
        \label{fig:gender_ratio_beforeLR0}
    \end{subfigure}
    %   \hspace{-16pt}
    \begin{subfigure}[b]{0.25\textwidth}
        \includegraphics[width=\linewidth]{figures/imSitu_mean_gender_ratio_test_50_013_01.pdf}
        \caption{Gender ratio on training and test with LR. }
        \label{fig:gender_ratio_afterLR0}
    \end{subfigure}
    
    \begin{subfigure}[b]{0.25\textwidth}
        \includegraphics[width=\linewidth]{figures/imSitu_dev_man_mean_verb_ratio0_03_001.pdf}
        \caption{Mean verb ratio  for man on training and dev without LR.}
        \label{fig:test_gender_ratio_beforeLR0}
    \end{subfigure}
    %   \hspace{-16pt}
    \begin{subfigure}[b]{0.25\textwidth}
        \includegraphics[width=\linewidth]{figures/imSitu_test_man_mean_verb_ratio0_03_001.pdf}
        \caption{mean gender ratio for man on training and test with LR. }
        \label{fig:test_gender_ratio_afterLR0}
    \end{subfigure}
    
        \begin{subfigure}[b]{0.25\textwidth}
        \includegraphics[width=\linewidth]{figures/imSitu_dev_woman_mean_verb_ratio0_03_001.pdf}
        \caption{Mean verb ratio  for woman on training and dev without LR.}
        \label{fig:test_gender_ratio_beforeLR0}
    \end{subfigure}
    %   \hspace{-16pt}
    \begin{subfigure}[b]{0.25\textwidth}
        \includegraphics[width=\linewidth]{figures/imSitu_test_woman_mean_verb_ratio0_03_001.pdf}
        \caption{mean gender ratio for woman on training and test with LR. }
        \label{fig:test_gender_ratio_afterLR0}
    \end{subfigure}
    \caption{Mean gender ratio} 
    \label{fig:imSitu_gender_ratio0}
\end{figure*}

Structured prediction models have been widely used in many NLP tasks, where the inter-dependencies between output variables can be explicitly defined. the imSitu vSRL system considers 
In this section, we will provide the description of the original inference problem using the semantic role labeling system imSitu as an example. 
In this system, when trying to get the prediction, we will calculate scores for different verbs as well as scores for different semantic role pairs (such as ``place" - ``room"). As we mentioned before, imSitu adopts the CRF model which will also provide a score for the relation between verbs and the semantic role pairs.

To generate the prediction for each instance in imSitu, there are some constraints:
\begin{compactitem}
    \item For all the candidate verbs, each time only one verb can be chosen.
    \item For one given verb, there can be several semantic role pairs, such as (``agent'' - ``people''), (``tool'' - ``shears'') and (``place'' - ``field''). 
\end{compactitem}

We use $s(x)$ to stand for the score of role $x$. We also define $y \in \{0,1\}$ to control if one element will be chosen. So the original problem can be defined as:

\begin{subequations}
\label{eq:ori}
\begin{align}
    \max_{y_v, y_{v,r}} & \quad {(\sum_v y_v s(v) + \sum_{v,r}y_{v,r}s(v,r))} \label{eq:obj} \\        
    \text{s.t.} 
        & \sum_v y_v = 1, \label{eq:oneverb}\\           
        & \sum_r y_{v,r} > 0 \Longrightarrow y_v = 1,  \forall v  \label{eq:vtor}
\end{align}
\end{subequations}
where $v$ stands for ``verb'', $r$ stands for the semantic role pairs. 
Eq~\eqref{eq:oneverb} means that at each time only one verb can be chosen. Eq~\eqref{eq:vtor} means that if some semantic role pairs for one verb $v$ are chosen in the prediction, this verb $v$ must also occur in the prediction.

In imSitu, different verbs can have different roles. We define  $\Omega(v,r)$ to stand for all the possible roles for the verb $v$. Each semantic role can be assigned with different objects, for example the role ``place''can be assigned with ``outdoor'', ``lake'' or ``field''. Different objects for this specific role will have different coefficients. The model will try to find the appropriate one among all the possible choices. So we can get the following constraint:
\begin{equation}
\sum_o y_{u,o} = 1, \quad \forall u \in \Omega(v,r)
\label{eq:rvso}
\end{equation}
where $o$ stands for the object and $u$ stands for the role of the corresponding verb $v$. Eq~\eqref{eq:rvso} means that for each role $u$, there will be only one object assigned to it.

Among all the possible objects for this specific role, there can be a null value. For example, given the verb ``cooking'' there shouldn't be any object  assigned to the role ``vehicle''. At this time, $y_{u,null} = 1$. But we can not assign all the roles with ``null'' for the chosen verb. So we get another constraint:

\begin{equation}
\forall v, \quad \sum_u y_{v,u,o^n} < |u| \Longrightarrow y_v =1
\label{eq:null_object}
\end{equation}
where $o^n$ means $object = null$.

With Eq~\eqref{eq:ori} to \eqref{eq:null_object}, the originial inference problem is now formulated as the integer linear programming problems. Next we will define our corpus-wise linear constraints and then adopt Lagrangian Relaxation algorithm to solve them which will be described in the following.

\subsection{Corpus-wise Constraints}

In imSitu, when doing the inference, we will predict one verb and correlated semantic role pairs for each instance. But sometimes we can not determine if  the predicted result is appropriate  for the specific instance. 
 For example, after the imSitu makes predictions for the randomly chosen image not in the dev data set, we do not know if the prediction is correct. Under this situation, we can make constraints on the whole corpus to prevent the prediction extremely biased to one direction. 

Previously we have defined our inference algorithm, but
Eq~\eqref{eq:ori} is the object function for one instance. In our work, we will consider on the whole corpus. So the modified object is 
\begin{equation}
 \max_{y^i_v, y^i_{v_r}}{\sum_i(\sum_v y^i_v s^i(v) + \sum_{v,r}y^i_{v,r}s^i(v,r))}
 \label{eq:con_obj}
\end{equation}
where $i$ stands for each instance in the corpus.
And the corpus-wise constraints can be written as linear functions:
\begin{equation}\label{eq:cor_cons}
 \sum_i(\sum_v y^i_v c^i(v) + \sum_{v,r}y^i_{v,r}c^i(v,r)) \leq a
\end{equation}
where $c^i(v)$, $c^i(v,r)$ and $a$ are the coefficients of the constraints. For example, if we set $c^i(v) = 1$, $c^i(v,r) = 0$ and $a = 20$, we make constraints that in our predictions, no more than 20 verbs can occur as the result. Note that all the coefficients are not dependent on instance $i$, so we can simplify the notations to $c(v)$ and $c(v,r)$.

As we mentioned above, we focus on decreasing the gender bias in modern semantic role labeling systems, besides constraints such as Eq~\eqref{eq:oneverb} and \eqref{eq:vtor}, we also make some corpus-wise constraints: we will add  margins to the gender ratio for each verb:
\begin{equation}\label{eq:cons_ratio}
 a_1 \leq \frac{\sum_i y^i_{v = v^*, r - m}}{\sum_i y^i_{v = v^*, r - w} + \sum_i y^i_{v = v^*, r - m}} \leq a_2
\end{equation}
where $a_1$ and $a_2$ are the lower bound and the upper bound of the gender ratio in corpus-wise predictions. $y^i_{v = v^*, r- m}$ means that ``$v^*$'' is the predicted verb and the combination (``agent'' - ``man'') will appear as one  semantic role pair. In Eq~\eqref{eq:cons_ratio}, ``m'' stands for ``man'' and ``w'' stands for ``woman''. The whole formula means that among all the predictions, for verb ``$v^*$'', the gender ratio is restricted to range $[a_1, a_2]$. In this work, we get $a_1$ and $a_2$ based on the training dataset. All the constraints generated from Eq~\eqref{eq:cons_ratio}  can be written in the form $Ay - b \leq 0$. Thus our object function is:

\begin{subequations}
\label{eq:objforlr}
\begin{align}
    \max_{y^i_v, y^i_{v_r}} & {\sum_i (\sum_v  y^i_v s^i(v)+\sum_{v,r}y^i_{v,r}s^i(v,r))} 
    \label{eq:objforlr1} \\        
& \text{s.t. } 
    A\sum_i y_{v,r}^i - b \leq 0, \label{eq:objforlr2}       
\end{align}
\end{subequations}
